# Supplementary material for: A Fractional Graph Laplacian Approach to Oversmoothing
Source: arXiv:2305.13084 source file (2023-10-31)
Supplement: Supplementary file 1 [file images_appendix.tex]

\section{Additional Images}
\label{sec:images}
% \begin{figure}[H]
%     \centering
%     \includegraphics{img/weakly_balanced.tikz}
%     \caption{
%     %Examples of non-weakly balanced (left), weakly balanced but not balanced (center), and balanced (right) directed graphs. The plot shows that balanced graphs are a proper subset of weakly balanced graphs and that non-weakly balanced graphs do exist. As the theory suggests, the Perron-Frobenius eigenvalue of the non-weakly balanced graph is $\lambda_\text{PF}\approx 0.986652\neq 1$. The Perron-Frobenius eigenvalue of both weakly balanced and balanced graphs is $\lambda_\text{PF}=1$, with corresponding $\mathbf{k}=(\sqrt{2}, 1, \sqrt{2}, \sqrt{2})\tran$ and $\mathbf{k}=(\sqrt{2}, 1, \sqrt{2}, \sqrt{1})\tran$, respectively. For this particular weakly balanced graph a stronger condition holds, namely, $a_{i, j} \(k_j/\sqrt{\smash[b]{d_j^\text{out}}}-k_i/\sqrt{d_i^\text{in}}\)=0$ for all $i, j \in\{1, \dots, 4\}$.
%     Examples of non-weakly balanced (left), weakly balanced (center), and balanced (right) directed graphs. The Perron-Frobenius eigenvalue of the left graph is $\lambda_\text{PF}\approx 0.97\neq 1$, while for the middle and right graphs $\lambda_\text{PF}=1$.
%     }
%     \label{fig:weakly_balanced}
% \end{figure}

\begin{figure}[H]
   \centering\includegraphics{img/evolution_chameleon.tikz}
    %\subfloat[Squirrel]{\includegraphics[width=.45\linewidth]{img/evolution_squirrel.tikz}}
   \caption{Simulation of the spectral evolution described in \cref{thm:normal_matrices} for the envelope of Chameleon spectra vs. real dynamics. In the left plot, we computed the envelope of eigenvalues of chameleon, and we evolved it according to the map $\lambda\mapsto\exp\(\iu \atan\(\Re \lambda, \Im \lambda\)\)\abs{\lambda}^\alpha$. In the right plot, we computed for each $\alpha$ the envelope of $\lambda\(\sna^\alpha\)\coloneqq\lambda\(\mathbf{U}\mathbf{\Sigma}^\alpha \mathbf{V}\herm\)$, which describes the real dynamics of the spectrum. The two plots would be roughly equal if the \acrshort{sna} of chameleon was a normal matrix.}
   \label{fig:directed_sna_spectrum}
\end{figure}
