# Supplementary material for: A Fractional Graph Laplacian Approach to Oversmoothing
Source: arXiv:2305.13084 source file (2023-10-31)
Supplement: Supplementary file 2 [file notation.tex]

\newacronym{fgl}{FGL}{Fractional Graph Laplacian}
\newacronym{ode}{ODE}{Ordinary Differential Equation}
\newacronym{gnn}{GNN}{Graph Neural Network}
\newacronym{svd}{SVD}{Singular Value Decomposition}
\newacronym{sna}{SNA}{Symmetrically Normalized Adjacency}
%\newacronym{snl}{SNL}{Symmetrically Normalized Laplacian}
\newacronym{fd}{FD}{Frequency Dominant}
\newacronym{lfd}{LFD}{Lowest Frequency Dominant}
\newacronym{hfd}{HFD}{Highest Frequency Dominant}
\newacronym{mlp}{MLP}{Multi-Layer Perceptron}
\newacronym{lcc}{LCC}{Largest Connected Components}
\newacronym{gcn}{GCN}{Graph Convolutional Network}
\newacronym{dsbm}{DSBM}{Directed Stochastic Block Model}
\newacronym{auroc}{AUROC}{Area under the ROC curve}
\newacronym{gat}{GAT}{Graph Attention Network}

\newglossaryentry{ImaginaryUnit}{
    type=symbols,
    name={\ensuremath{\iu}}, 
    description={Imaginary unit},
    sort=0
}
\newglossaryentry{ImaginaryPart}{
    type=symbols,
    name={\ensuremath{\Re(z)}}, 
    description={Real part of $z\in\mathbb{C}$},
    sort=0
}
\newglossaryentry{RealPart}{
    type=symbols,
    name={\ensuremath{\Im(z)}}, 
    description={Imaginary part of $z\in\mathbb{C}$},
    sort=0
}
\newglossaryentry{diag}{
    type=symbols,
    name={\ensuremath{\diag(\mathbf{x})}}, 
    description={Diagonal matrix with $\mathbf{x}$ on the diagonal.},
    sort=1
}
\newglossaryentry{allOnes}{
    type=symbols,
    name={\ensuremath{\mathbf{1}}}, 
    description={Constant vector of all $1$s.},
    sort=1
}
\newglossaryentry{Transpose}{
    type=symbols,
    name={\ensuremath{\mathbf{M}\tran}}, 
    description={Transpose of $\mathbf{M}$},
    sort=2
}
\newglossaryentry{Conjugate}{
    type=symbols,
    name={\ensuremath{\mathbf{M}\conj}},
    description={Conjugate of $\mathbf{M}$},
    sort=3
}
\newglossaryentry{ConjugateTranspose}{
    type=symbols,
    name={\ensuremath{\mathbf{M}\herm}},
    description={Conjugate transpose of $\mathbf{M}$},
    sort=4
}
\newglossaryentry{SpectralNorm}{
    type=symbols,
    name={\ensuremath{\norm{\mathbf{M}}}},
    description={Spectral norm of $\mathbf{M}$},
    sort=5
}
\newglossaryentry{FrobeniusNorm}{
    type=symbols,
    name={\ensuremath{\norm{\mathbf{M}}_2}},
    description={Frobenius norm of $\mathbf{M}$},
    sort=6
}
\newglossaryentry{Spectrum}{
    type=symbols,
    name={\ensuremath{\lambda\(\mathbf{M}\)}},
    description={Spectrum of $\mathbf{M}$},
    sort=7
}
\newglossaryentry{SingularValues}{
    type=symbols,
    name={\ensuremath{\sigma\(\mathbf{M}\)}},
    description={Singular values of $\mathbf{M}$},
    sort=8
}
\newglossaryentry{DirichletEnergy}{
    type=symbols,
    name={\ensuremath{\dir\(\mathbf{x}\)}},
    description={Dirichlet energy computed on $\mathbf{x}$},
    sort=9
}
\newglossaryentry{Homophily}{
    type=symbols,
    name={\ensuremath{\homophily\(\mathcal{G}\)}},
    description={Homophily coefficient of the graph $\mathcal{G}$},
    sort=10
}
\newglossaryentry{KroneckerProduct}{
    type=symbols,
    name={\ensuremath{\mathbf{A}\otimes \mathbf{B}}},
    description={Kronecker product between $\mathbf{A}$ and $\mathbf{B}$},
    sort=11
}
\newglossaryentry{Vectorization}{
    type=symbols,
    name={\ensuremath{\ve\(\mathbf{M}\)}},
    description={Vector obtained stacking columns of $\mathbf{M}$.},
    sort=12
}

% \newglossaryentry{PerronFrobeniusEigenvalue}{type=symbols,name={\ensuremath{\lambda\(\mathbf{M}\)_\text{PF}}},
% description={Perron-Frobenius eigenvalue of $\mathbf{M}$}}
